# Supplementary material for: A tunable plasmonic resonator using kinetic 2D inductance and patch capacitance
Source: arXiv:2011.09142 source file (2020-11-18)
Supplement: Supplementary file 1 [file Supplemental.pdf]

# Supplementary Material for
# "A tunable plasmonic resonator using kinetic 2D inductance and patch capacitance"


V. M. Muravev*, N. D. Semenov, I. V. Andreev, P. A. Gusikhin, I. V. Kukushkin

*Institute of Solid State Physics, RAS, Chernogolovka, 142432 Russia*



(Dated: November 18, 2020)


## I. CAPACITANCE AND INDUCTANCE MODELING

The capacity and inductance calculations were performed using the 3D electromagnetic analysis software. The model describes electromagnetic response of the $4 \times 4 \times 0.55$ mm$^3$ gallium arsenide chip with 30 nm wide quantum well placed at a depth of $h = 440$ nm below the crystal surface. The electron density in the two-dimensional electron system (2DES) was $n_s = 2 \times 10^{11}$ cm$^{-2}$ with the mobility $2 \times 10^6$ cm$^2$/V·s. Gold contacts of different sizes and shapes are placed on the top surface of the substrate and partially cover the 2DES (Fig. S1).

According to the assumption of the model, for calculation of the inter-contact capacitance $C$ we exclude 2DES from consideration and calculate lateral capacitance between the contacts. The constructed object was placed in a non-conductive medium with open boundary conditions. A small potential difference was applied between the gold contacts. After that, the electrostatic problem was solved on an uneven tetrahedral mesh (this was an option due to the very different spatial dimensions of the various components of the system) consisting of about 400000-500000 meshcells. This model gives 0.1% accuracy. Figure S1(a) shows the example of the calculated potential distribution in the sample with $0.85 \times 0.7$ mm$^2$ contact size. The distance between contacts was 0.5 mm. The simulation gave a capacitance value of $C = 0.115$ pF.

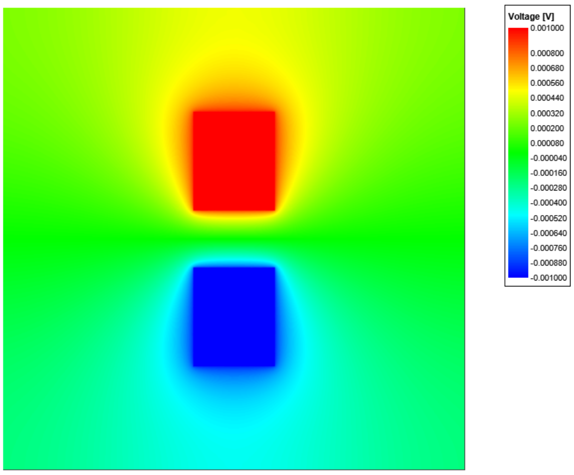


(a)

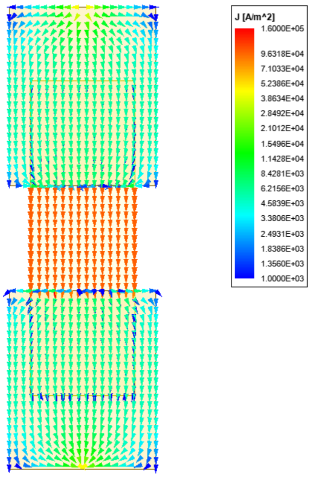


(b)

FIG. S1: (a) Calculated electric field potential distribution in the sample when applying voltage between the contacts. (b) Calculated current distribution in the contacts and 2DES (in logarithmic scale for clarity).

For the magnetic inductance ($L$) calculation, we modeled the structure in which the contacts are connected to each other via the 2DES (Fig. S1(b)). A constant current was passed through the system. Wires with diameter of 20 $\mu$m were connected to the opposite sides of the structure. They served as a source and a sink for the current. The problem was solved on an uneven tetrahedral mesh consisting of about 450000 meshcells giving 0.1% accuracy. Figure S1(b) shows the example of the calculated current distribution in the sample $0.85 \times 0.7$ mm$^2$ contact size. The contacts are connected by $0.5 \times 0.5$ mm$^2$ two-dimensional electron system. The simulation gave the magnetic inductance value of $L = 1.7$ nH.

---


* Corresponding E-mail: muravev@issp.ac.ru

## II. DETAILED DRAWINGS FOR STRUCTURES WITH DIFFERENT CONTACT GEOMETRY

Figure 2 shows detailed drawings for samples with contact size $0.4 \times 0.7$ mm$^2$ (sample 1) and $1.1 \times 3.9$ mm$^2$ (sample 2). The modeling yields the following values of inter-contact capacitance $C = 7.5 \times 10^{-2}$ pF (sample 1), and $C = 0.91$ pF (sample 2). The magnetic inductance for these samples was $L = 1.06$ nH (sample 1), and $L = 1.48$ nH (sample 2).

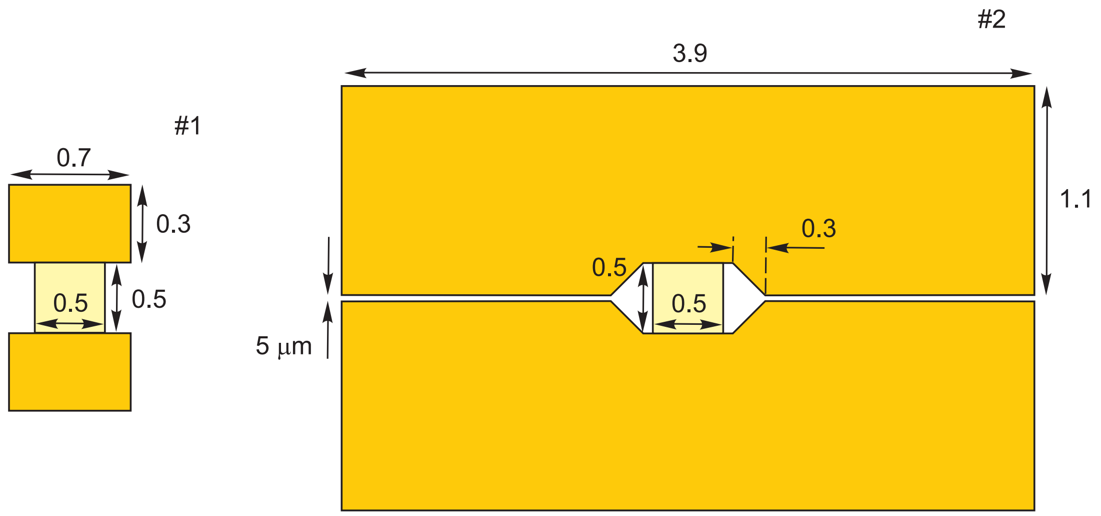


FIG. S2: Detailed drawings for samples with contact size $0.3 \times 0.7$ mm$^2$ (sample 1) and $1.1 \times 3.9$ mm$^2$ (sample 2). Unless otherwise specified, all dimensions are in millimeters.
